# Supplementary material for: Deterministic Tree Embeddings with Copies for Algorithms Against Adaptive Adversaries
Source: arXiv:2102.05168 source file (2021-02-09)
Supplement: Supplementary file 1 [file appendix.tex]

\section{Scrap / Things That Weren't Needed}
	
		\subsubsection{A Node-Weighted Version of The FRT Cutting Scheme}
	
	In order to give our deterministic construction we must unpack the black box of the \citet{fakcharoenphol2004tight} cutting scheme. 
	
	The \citet{fakcharoenphol2004tight} cutting scheme given metric $(V, d)$ where $d(u,v) \geq 1$ for all $u,v \in V$ produces a hierarchical decomposition $\mcH = \{\mcP_0, \ldots, \mcP_h\}$ and is as follows. We first pick a uniformly random permutation $\pi$ on $V$ and a uniformly random value $\beta \in [\frac{1}{2}, 1)$. We let the radius for level $i$ be $r_i := 2^{i-1} \cdot \beta$.
	
	We let $\mcP_h$ be the trivial partition containing all vertices of $V$. Next, we construct $\mcP_{i}$ by refining $\mcP_{i+1}$; in particular we divide each part $P_{i+1} \in \mcP_{i+1}$ into additional parts as follows. Each $v \in P_{i+1}$ is assigned to the first vertex $u$ in $\pi$ for which $v \in B(u, r_i)$. Notice that $u$ need not be in $P_{i+1}$. Let $C_u$ be all vertices in $P_{i+1}$ which are assigned to $u$ and add to $\mcP_i$ all $C_u$ which are non-empty.
	
	One can easily verify that the resulting partitions indeed form a hierarchical decomposition.

	We slightly modify the FRT cutting scheme to account for node weights. In particular, consider the \citet{fakcharoenphol2004tight} cutting scheme as described above but where a node's position in $\pi$ is chosen proportional to its weight in some probability distribution $p$ over $V$. In particular, $\pi$ can be thought of as being iteratively constructed as follows: Suppose $\pi$ is an ordering on nodes $V' \subseteq V$; then, letting $\bar{V} = V \setminus V'$, $v \in \bar{V}$ is selected as the next node in $\pi$ with probability $p_v / \sum_{u \in \bar{V}} p_u$; we repeat this process until $\pi$ is an ordering on all nodes in $V$ and therefore a permutation on $V$. 
	
	\begin{lemma}\label{lem:permOrder}
		Given the node-weighted random permutation, $\pi$, computed as above, the probability that node $u$ precedes all nodes in $V' \subseteq V$ in $\pi$ is $p_u / p(V')$ where $p(U) := \sum_{w \in V'} p_w$.
	\end{lemma}
	\begin{proof}
		\todo
	\end{proof}
	
	Moreover, whereas the original \citet{fakcharoenphol2004tight} makes use of the fact that $H_n := \sum_{i=1}^n \frac{1}{i} \leq O(\log n)$, because we are dealing with node weights we will have to prove a slight generalization of this fact which takes node weights into account. In particular we prove the following lemma which implies $H_n \leq O(\log n)$ when all $p^{(i)}$ are equal.
	\begin{lemma}\label{lem:harmGen}
		Let $p^{(1)}, \ldots, p^{(n)}$ be real numbers where $p^{(i)} > 0$, $\sum_i p^{(i)} = 1$ and $p^{(1)} \geq \frac{1}{\poly(n)}$. Then
		\begin{align*}
		\sum_{i=1}^n \frac{p^{(i)}}{\sum_{j \leq i}p^{(j)}} \leq O(\log n).
		\end{align*}
	\end{lemma}
	\begin{proof}
		Let $t_i := \sum_{j \leq i}p^{(j)}$ be the total mass contained in the first $i$ reals; i.e.\ we would like to show $\sum_{i=1}^n \frac{p^{(i)}}{t_i} \leq O(\log n)$. We know $t_n = 1$ and initially $t_1 \geq \frac{1}{\poly(n)}$. Our strategy will be to show that a large term in $\frac{p^{(i)}}{\sum_{j \leq i}p^{(j)}}$ causes a large multiplicative increase from $t_{i-1}$ to $t_i$ which, given the fact that $t_n = 1$, cannot happen too often.
		
		More formally, we have the following identity
		\begin{align*}
		t_i = t_{i-1} + p^{(i)} = t_{i-1} \left(1 + \frac{p^{(i)}}{t_{i-1}} \right).
		\end{align*}
		Rearranging this we find that
		\begin{align}\label{eq:ratioOfTotal}
		\frac{t_i}{t_{i-1}} = \left(1 + \frac{p^{(i)}}{t_{i-1}} \right).
		\end{align}
		
		Using a telescoping product and $t_n = 1$, we have that
		\begin{align*}
		1 = t_n = t_1 \cdot \frac{t_2}{t_1} \cdot \frac{t_3}{t_2} \ldots \frac{t_n}{t_{n-1}}
		\end{align*}
		which when combined with \Cref{eq:ratioOfTotal} and the fact that $t_1 = p^{(1)} \geq \frac{1}{n^c}$ for some constant $c>0$ gives
		\begin{align*}
		\frac{1}{t_1} &= \cdot \prod_{i=2}^n \left[ 1 + \frac{p^{(i)}}{t_{i-1}} \right] \\
		c \cdot \log n  &\geq  \sum_{i=1}^n \left[ \log\left(1 + \frac{p^{(i)}}{t_{i-1}}\right)\right]
		\end{align*}
		Using the fact that $\log(1+x) \geq \frac{x}{2}$ for $x \in [0, 2]$ and flipping our inequality we have $\sum_{i=2}^n \frac{p^{(i)}}{t_{i-1}} \leq 2c \cdot \log n $. Finally, using the fact that $t_{i-1} \leq t_{i}$, we have
		\begin{align*}
		\sum_{i=1}^n \frac{p^{(i)}}{t_i} &= 1 + \sum_{i=2}^n \frac{p^{(i)}}{t_i}\\
		& \leq 1 + \sum_{i=2}^n \frac{p^{(i)}}{t_{i-1}}\\
		& \leq 1 + 2c \cdot \log n = O(\log n),
		\end{align*}
		as desired.

	\end{proof}
	
	\subsubsection{Derandomizing via Multiplicative Weights}
	
	As discussed above, our goal is to derandomize \Cref{lem:FRTIsPadded} while taking node weights into account. 
	
	We are now ready to formalize our node-weighted derandomization. 
	
	\begin{lemma}\label{lem:derandPadding}
		There is a deterministic algorithm which given metric $(V, d)$ and a distribution over nodes $p_v$ returns a hierarchical decomposition $\mcH$ in which at least a $.95$ fraction of nodes are $\frac{1}{\log n}$-padded by weight; i.e. 
		\begin{align*}
		\sum_v p_v \cdot \mathbb{I}\left(\text{$v$ is $\Omega\left(\frac{1}{\log n}\right)$-padded in $\mcH$}\right)\geq .95.
		\end{align*}
	\end{lemma}
	\begin{proof}
		The analysis will be similar to that of \citet{fakcharoenphol2004tight} and \citet{gupta2006oblivious} with slight modifications to account for node-weights; in particular, we will make use of \Cref{lem:harmGen}.
		
		Now, given $\pi$ selected in this fashion, run the \citet{fakcharoenphol2004tight} cutting scheme as above to get a hierarchical decomposition $\mcH$.
		
		We first claim that this process pads a large fraction of nodes by weight. In particular, we claim that
		\begin{align}
		\E_{\pi, \beta}\left[\sum_v p_v \cdot \mathbb{I}(\text{$v$ is $\alpha$-padded in $\mcH$})\right] \geq .95.
		\end{align}
		for $\alpha = \frac{c'}{\log n}$ for constant $c' > 0$ to be chosen later.
		
		Fix a node $v$. We will show that for each $i$, the ball $B_i := B(v, \alpha 2^i)$ is cut with sufficiently small probability and then show, by a union bound, that for a fixed $v$ the probability that $B_i$ is cut for some $i$ is at most $.05$.
		
		Say that node $u$ \emph{protects} $B_i$ if its ball at level $i$ contains $B_i$, i.e.\ if $r_i \geq d(u,v) + 2^i \alpha$. Say that $u$ \emph{threatens} $B_i$ if its ball at level $i$ intersects $B_i$ but does not contain it, i.e.\ $d(u,v) - \alpha 2^i < r_i < d(u,v) + 2^i \alpha$. Finally, say that $u$ \emph{cuts} $B_i$ if it threatens $B_i$ and is the first node in $\pi$ to threaten or protect $B_i$. Clearly if $B_i$ is not cut by any node for all $i$ then $v$ will be $\alpha$-padded. 
		
		In order for $B_i$ to be cut by $u$ it must be the case that $u$ threatens $B_i$ and no node before $u$ in $\pi$ threatens or protects $B_i$. By how we choose $r_i$, $u$ threatens $B_i$ if 
		\begin{align}
		d(u,v) - 2^i \alpha < \beta \cdot 2^{i-1} < d(u,v) + 2^i \alpha
		\end{align}
		and since $\beta \cdot 2^{i-1}$ is distributed uniformly in $[2^{i-2}, 2^{i-1})$, this happens with probability $2^{i+1}\alpha/2^{i-2} = 8\alpha$.
		In order for $u$ to be the first node to threaten or protect $B_i$, it certainly must be the case that every node which is closer to $v$ than $u$ appears after $u$ in $\pi$ (since every such node either threatens or protects $B_i$). Letting, $N_v(u) := \{w \in V : d(w, v) \leq d(u,v) \}$ be all nodes as close to $v$ as $u$, by \Cref{lem:permOrder} we have that this happens with probability $p_u / p(N_v(u))$ where $p(N_v(u)) := \sum_{w \in N_v(u)} p_w$. 
		
		Lastly, a node which is too far or too close to $v$ cannot cut $B_i$. In particular, a node $u$ can only cut $B_i$ if 
		\begin{align*}
		2^{i-2} - 2^i \alpha \leq d(u,v) \leq 2^{i-1} +2^i \alpha
		\end{align*}
		
		%Thus, we let $L := \{u : d(u,v) \leq 2^{i-2} - \frac{2^i}{\log n} \}$ be all nodes too close to $v$ to cut it and let  $p_L := \sum_{u \in L}p_u$ be the probability mass on these nodes.
		
		We let $C_i := \{u : 2^{i-2} - 2^i \alpha \leq d(u,v) \leq 2^{i-1} + 2^i\alpha \}$ be all such nodes which might cut $B_i$.
		
		Thus, we have that the probability that $B_i$ is cut is at most
		\begin{align*}
		\sum_{u \in C_i} \Pr(\text{$u$ precedes all $w \in N_v(u)$ in $\pi$ where $w \neq u$}) \cdot \Pr(\text{$u$ threatens $B_i$}) \leq \sum_{u \in C_i} \frac{p_u}{p(N_v(u))} \cdot 8 \alpha
		\end{align*}
		
		Thus, by a union bound the probability that some $B_i$  centered around $v$ for some $i$ is cut is at most
		\begin{align*}
		8 \alpha \sum_i \sum_{u \in C_i} \frac{p_u}{p(N_v(u))}
		\end{align*}

		Next, we claim that each $u$ occurs in at most $3$ of the $C_i$. \todo 
		
		Thus, letting $p^{(l)} = p_u$ where $u$ is the $l$th closest node to $v$ we have that the probability that some $B_i$ centered around $v$ is cut is at most
		\begin{align*}
		24 \alpha \sum_l \frac{p^{(l)}}{\sum_{j \leq l}p^{(j)}}.
		\end{align*}	
		
		Applying \Cref{lem:harmGen} we know $\frac{p^{(l)}}{\sum_{j \leq l}p^{(j)}} \leq c \cdot \log n$ for some constant $c > 0$ and so we conclude that this is at most
		\begin{align*}
		24 c \cdot \alpha \cdot \log n = \frac{24 c}{c'}
		\end{align*}
		which for $c'$ sufficiently small is at most $.05$.
		
		We now use the method of conditional expectation to derandomize this process.

		\todo
	\end{proof}
	
	Using the above node-weighted derandomization lemma gives our deterministic repetition HST construction. In particular, we run the following multiplicative-weights-type algorithm with $\epsilon = .01$ and set the number of iterations as $T:=4 \ln n / \epsilon^2$. In the following we let $p_v^{(t)} : = w^{(t)}_v / \sum_v w_v^{(t)}$ be the proportional share of $v$'s weight in iteration $t$.
	
	\begin{enumerate}
		\item Uniformly set the initial weights: $w_v^{(1)}=1$ for all $v \in V$.
		\item For $t \in [T]$:
		\begin{enumerate}
			\item Run the algorithm given in \Cref{lem:derandPadding} using distribution $p^{(t)}$ and let $\mcH_t$ be the resulting hierarchical decomposition.
			\item \textbf{Set mistakes:} For each vertex $v$ which is $\frac{1}{\log n}$-padded in $\mcH_t$ let $m_v^{(t)} = 1$. Let $m_v^{(t)} = 0$ for all other $v$.
			\item \textbf{Update weights:} for all $v \in V$, let $w_v^{(t+1)} \gets \exp(-\epsilon m_v^{(t)}) \cdot w_v^{(t)}$.
		\end{enumerate}
		\item Return $(\mcH_t)_t$.
	\end{enumerate}
	
	We state a well-known fact regarding multiplicative weights in our notation. Readers familiar with multiplicative weights may recognize this as the fact that the expected performance of mutliplicative weights over logarithmically-many rounds is competitive with the best expert.
	
	\begin{lemma}[\cite{arora2012multiplicative}]\label{lem:MWAvg}
		The above algorithm guarantees that for any $v \in V$ we have
		\begin{align*}
		\frac{1}{T} \sum_{t \leq T} p^{(t)} \cdot m^{(t)} \leq \epsilon + \frac{1}{T} \sum_{t \leq T} m_v^{(t)}
		\end{align*}
		where $p^{(t)} \cdot m^{(t)} := \sum_v p^{(t)}_v m_v^{(t)}$ is the usual inner product.
	\end{lemma}

	Using this fact we conclude that the above algorithm gives a $(\log n, \log n)$-repetition HST.
	\begin{lemma}
		There is a deterministic polynomial time algorithm which returns a $(\log n, \log n)$-repetition HST.
	\end{lemma}
	\begin{proof}
		We let the repetition HST's trees be the trees corresponding to $(\mcH_t)_t$ and we let the good nodes of the tree corresponding to $\mcH_t$ be the nodes which are $\Omega(\frac{1}{\log n})$-padded in $\mcH_t$. 
		
		Each tree corresponding to each $\mcH_t$ is a tree-embedding by construction and by \Cref{lem:padGivesDist} the distances between all good nodes are preserved up to an $O(\log n)$ stretch as required. Since $T:=4 \ln n / \epsilon^2$ we know that $T = O(\log n)$. 
		
		We need only argue, then, that each node is good in at least a $.9$ fraction of the $T$ total $\mcH_t$. Let $f_v = \frac{1}{T} \sum_{t \leq T} \mathbb{I}(\text{$v$ $\Omega(\frac{1}{\log n})$-padded in $\mcH_t$})$ be the fraction of the trees in which $v$ is good. Consider a fixed node $v$. By \Cref{lem:MWAvg} we know that 
		\begin{align}\label{eq:mwguar}
		\frac{1}{T} \sum_{t \leq T} p^{(t)} \cdot m^{(t)} \leq \epsilon + \frac{1}{T} \sum_{t \leq T} m_v^{(t)}
		\end{align}
		
		By definition of $m_v^{(t)}$ we have that the right hand side of \Cref{eq:mwguar} is $\epsilon + f_v$. On the other hand, by how we set $m^{(t)}$, the left hand side of \Cref{eq:mwguar} is $\frac{1}{T}\sum_t\sum_v p_v \cdot \mathbb{I}(\text{$v$ is $\frac{1}{\log n}$-padded in $\mcH$})$ which by \Cref{lem:derandPadding} is at least $.95$. Combining these facts we have $.95 \leq \epsilon + f_v$ and so by our choice of $\epsilon$ we know $.9 \leq f_v$.
	\end{proof}
